# Supplementary material for: All-water supercapacitor enabled by 1-nm clay channels
Source: arXiv:2410.11983 source file (2026-03-06)
Supplement: Supplementary file 1 [file supplement.pdf]

## 1. Supplementing figures

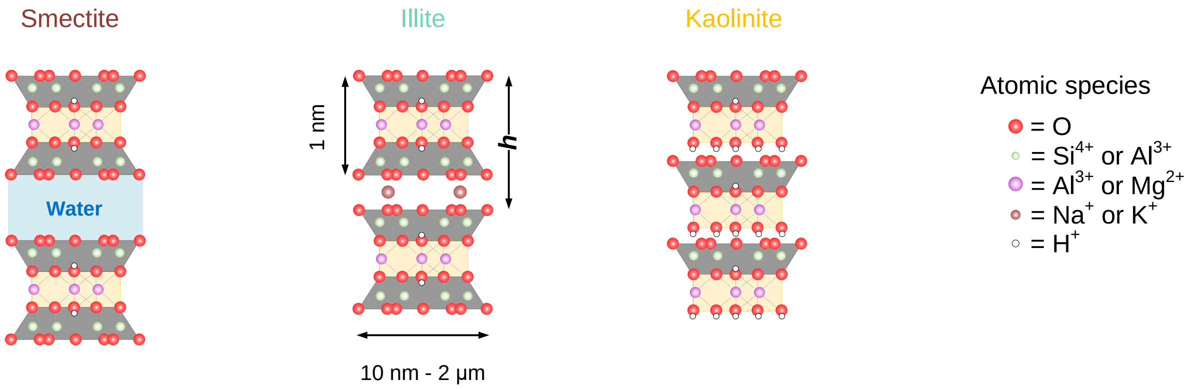


**Fig. S1.** Atomic structure of the three most common clays.

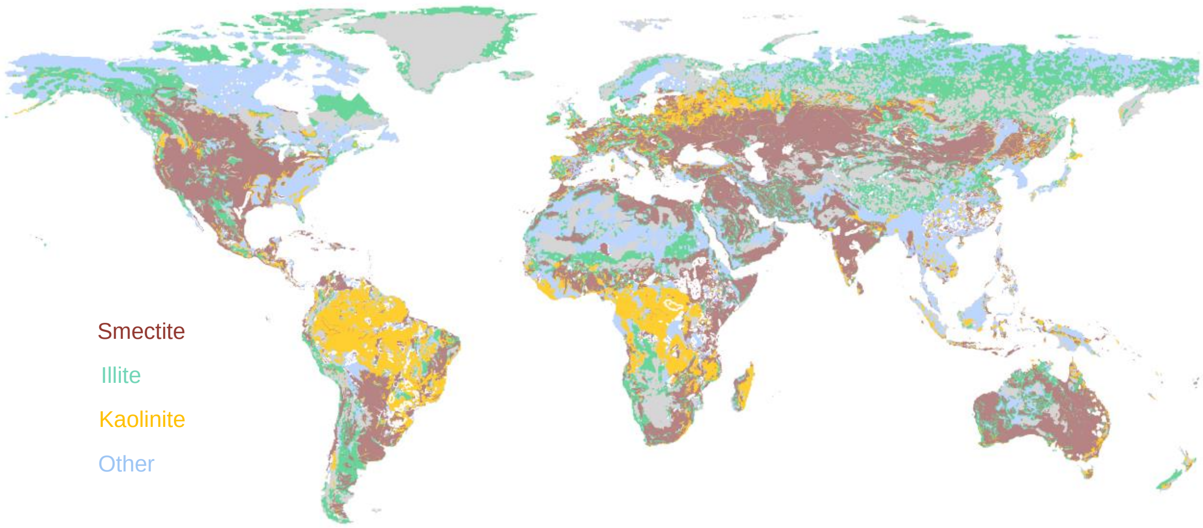


**Fig. S2.** Topsoil clay distribution map (data [4]) depicting regions with areal density of clay exceeding 10 kg/m$^2$.

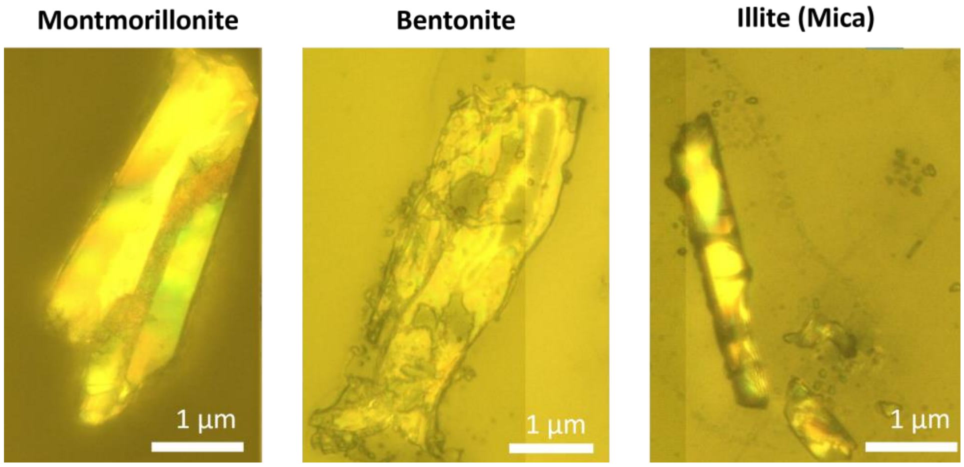


**Fig. S3.** Optical photos of large clay crystals of montmorillonite, bentonite, and illite, from left to right, respectively.

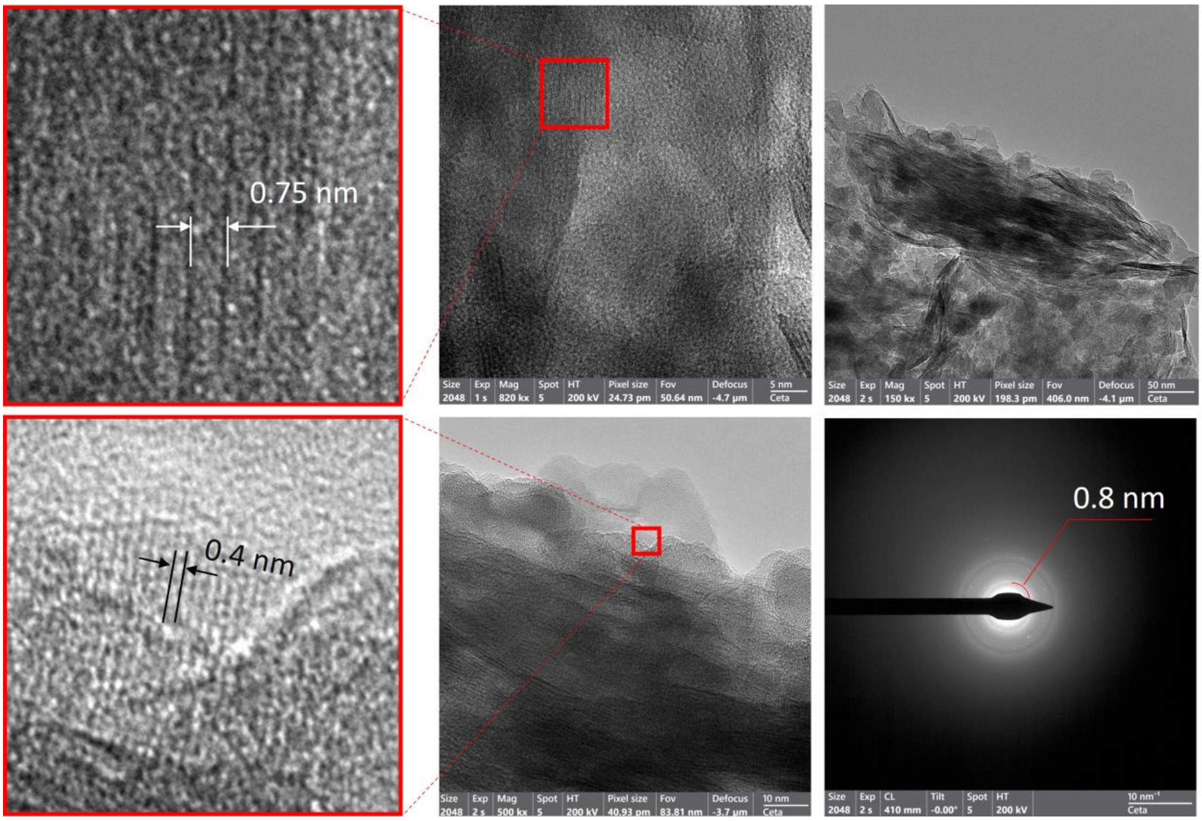


**Fig. S4.** Transmission electron microscopy (TEM) images and selected area electron diffraction (SAED) pattern of montmorillonite (MMT) crystals.

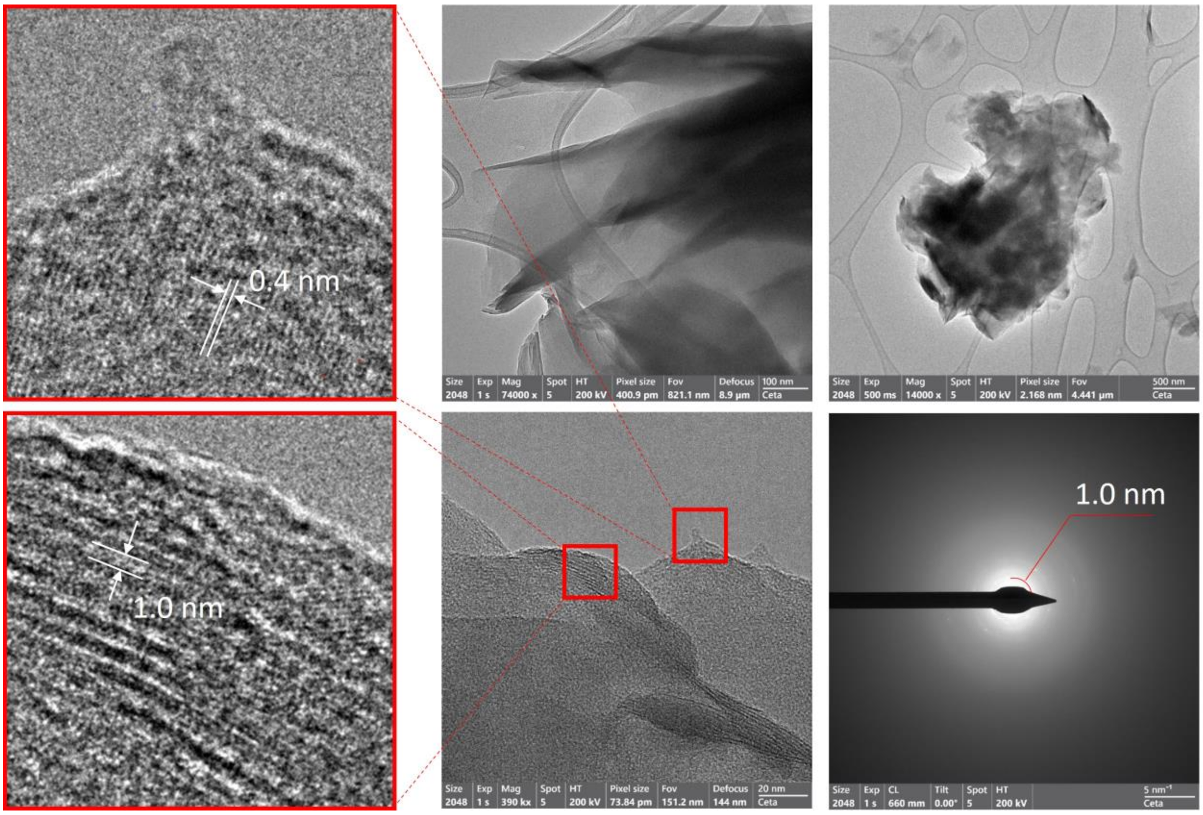


**Fig. S5.** The same as in Fig. S4 but for bentonite crystals.

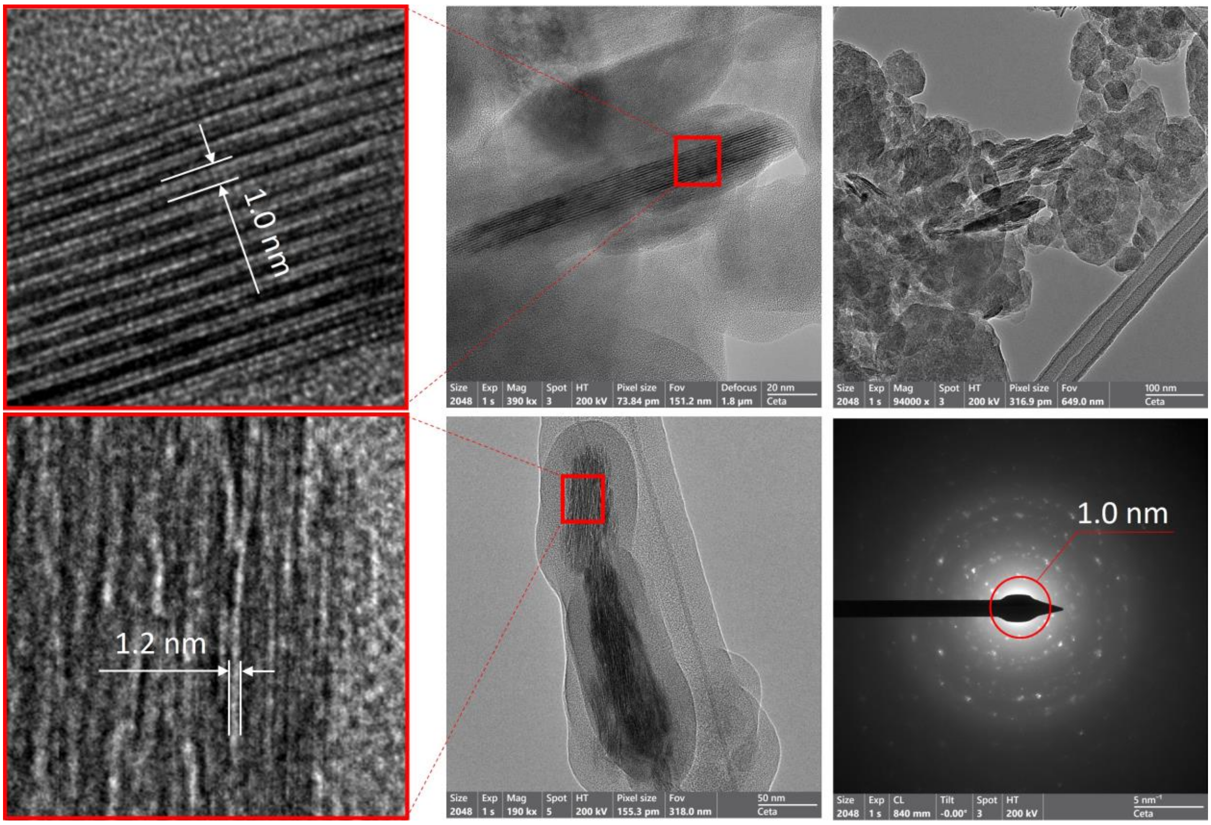


**Fig. S6.** The same as in Fig. S4 and S5 but for illite crystals.

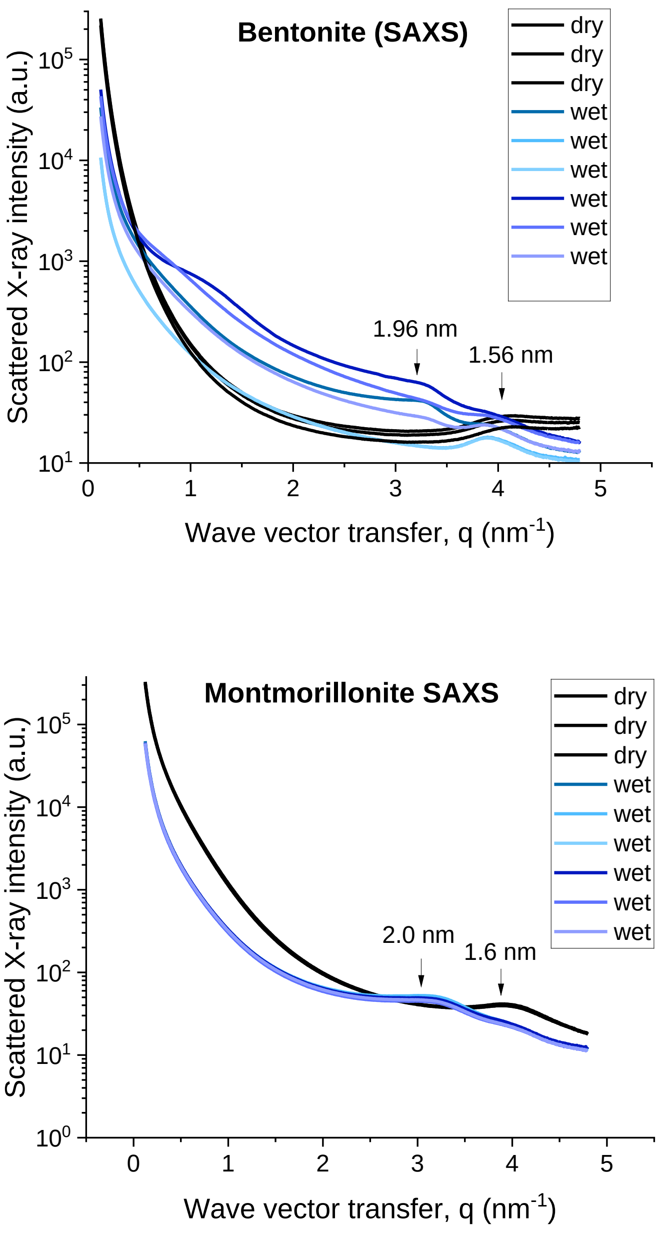


**Fig. S7. Small-angle X-ray scattering** (SAXS) of wet and dry bentonite (top) and montmorillonite (bottom) clay powders, recorded at the P62 SAXS/WAXS beamline of the PETRA III synchrotron source. The numbers next to the arrows indicate the interlayer distances corresponding to the peak maxima in reciprocal space. Note that the semi-dry sample was stored in a low-humidity environment without vacuum or annealing, resulting in a larger interlayer distance compared to the vacuum-dried TEM samples in Figs. S4–S6.

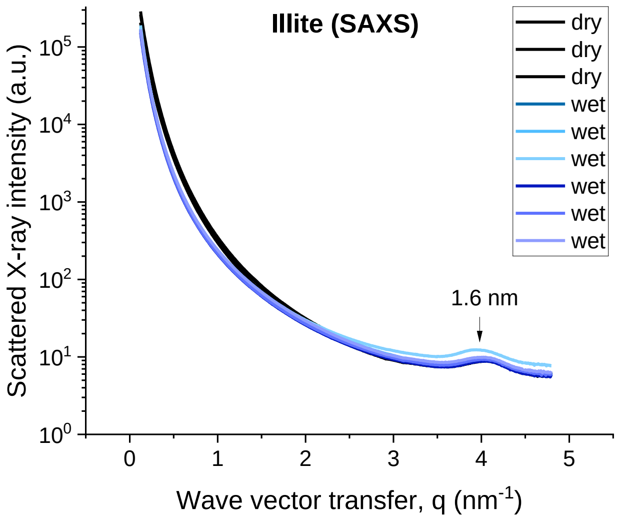


**Fig. S8.** Same as in Fig. S7 for illite clay powders. No diffraction peak shift indicates no water penetration between the crystalline layers (see Fig. 3b of the main text).

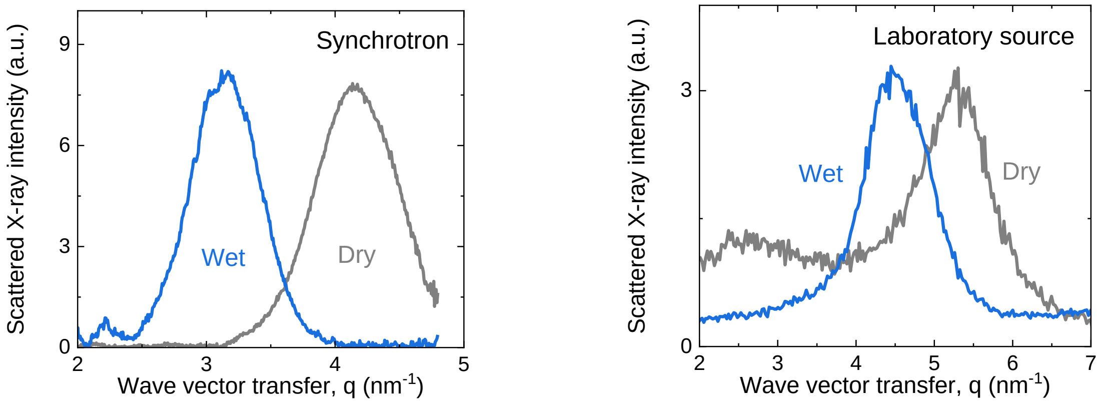


**Fig. S9. Small-angle X-ray scattering** (SAXS) of wet and dry bentonite clay powders. The data show the first diffraction peak. The graph on the left is synchrotron data (Fig. S7 with subtracted baseline). The samples were immersed in liquid water. The data on the right is Bruker XRD laboratory source measurements. The samples were prepared in saturated water vapor. The shift of the peaks in both measurements confirms water penetration between the bentonite clay crystal layers.

**Table S1.** ξ-potentials (in mV) of the nano-colloidal solutions of different clay types and graphene in pure 18-MΩ water with a pH of 7. Measurements were done with Malvern Panalytical™ Zetasizer.

| Meas. number | Smectite (MMT) | Kaolinite | Illite | Graphene |
|---|---|---|---|---|
| 1 | -30.9 | -17.2 | -15.2 | -16.2 |
| 2 | -31.7 | -16.4 | -16.6 | -15.5 |
| 3 | -30.6 | -16.7 | -15.2 | -14.9 |
| Average | -31.1 | -16.8 | -15.7 | -15.5 |

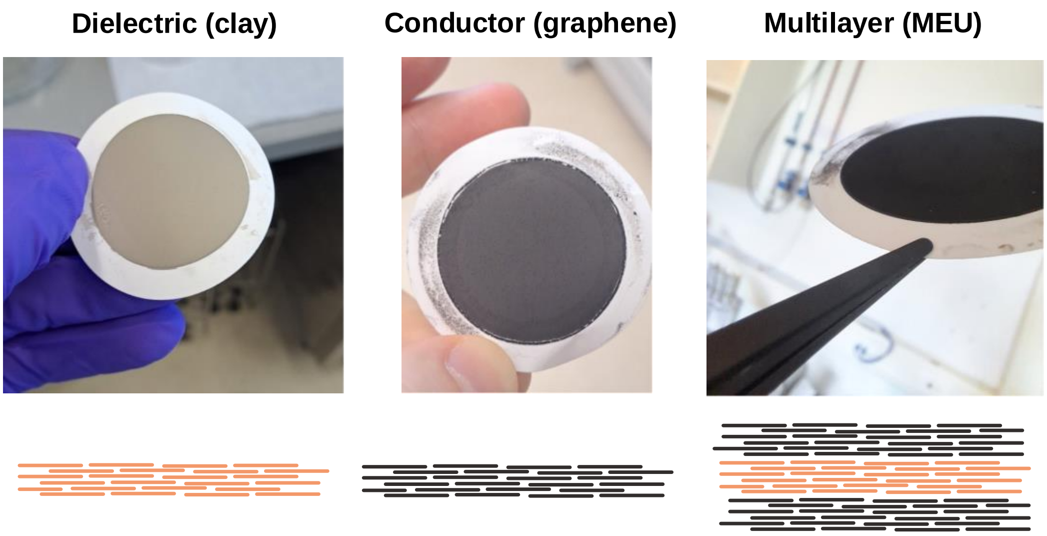


**Fig. S10. Van der Waals heterostructures** made in this study. Ø3.5-cm film membranes of clay (left), graphene (middle), and a multilayer graphene-clay-graphene membrane-electrode unit (MEU). The bottom sections schematically illustrate the structure of the films, where a stick represents a 2D crystal of the original material. These crystals are unidirectionally oriented and held together by van der Waals forces, providing enhanced flexibility and mechanical stability compared to compressed clay-based structures.

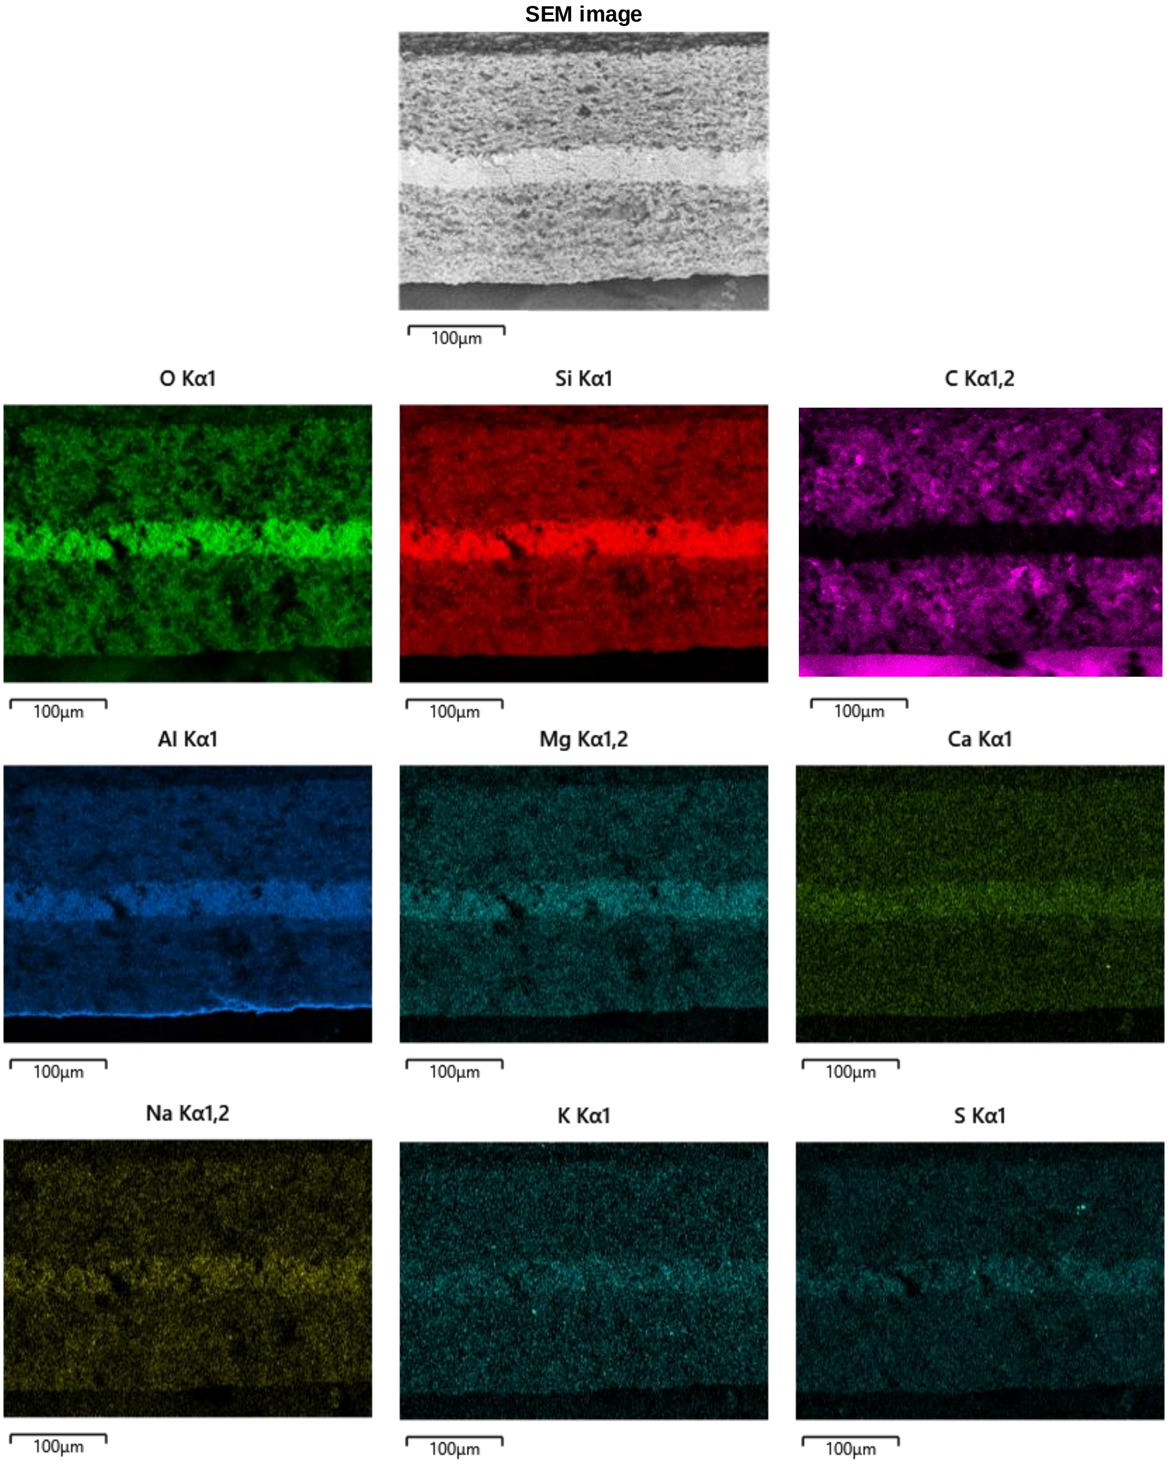


**Fig. S11.** SEM energy dispersive X-ray (EDX) element mapping for a cross-section of a membrane-electrode unit (MEU) made of smectite clay and graphene. Color maps are associated with the chemical species expected in the system (O, Si, C, Al, and Mg), in agreement with crystal structure, plus traces of Ca, Na, K, and S. The top is the SEM micrograph. The EDX sum spectrum of the element mapping is shown in Fig. S12.

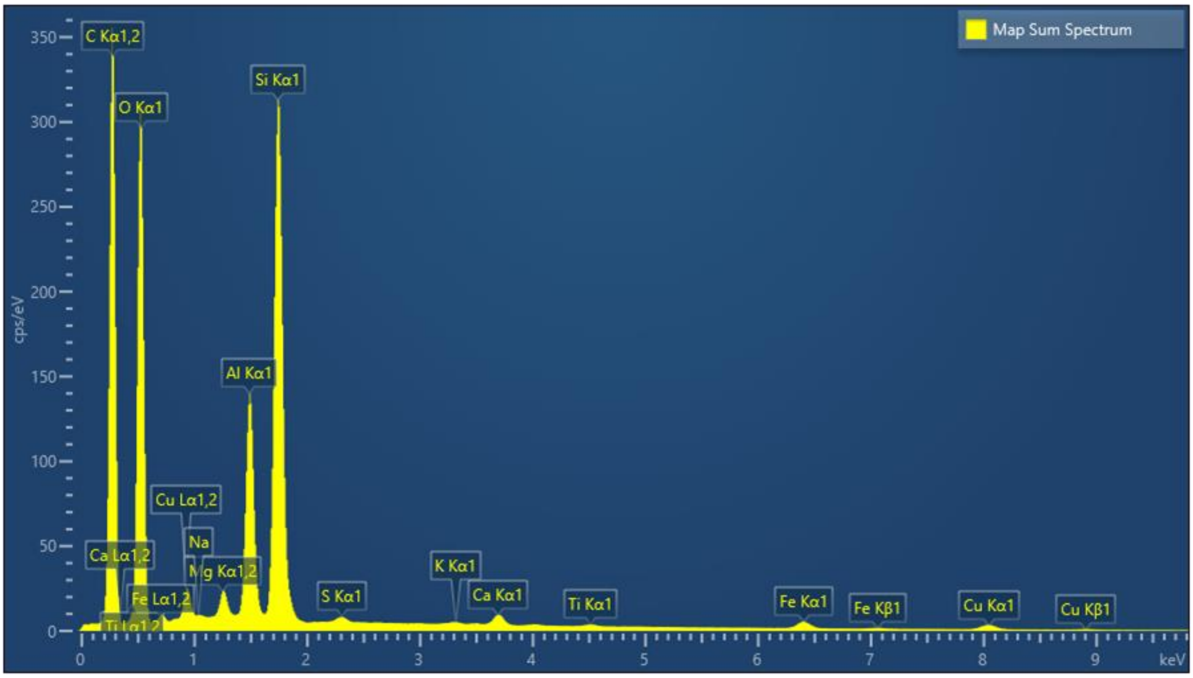


**Fig. S12. EDX sum spectrum** associated with the elemental map shown in Fig. S11. The spectrum indicated the presence of the chemical species composing the clay crystal structure, alone.

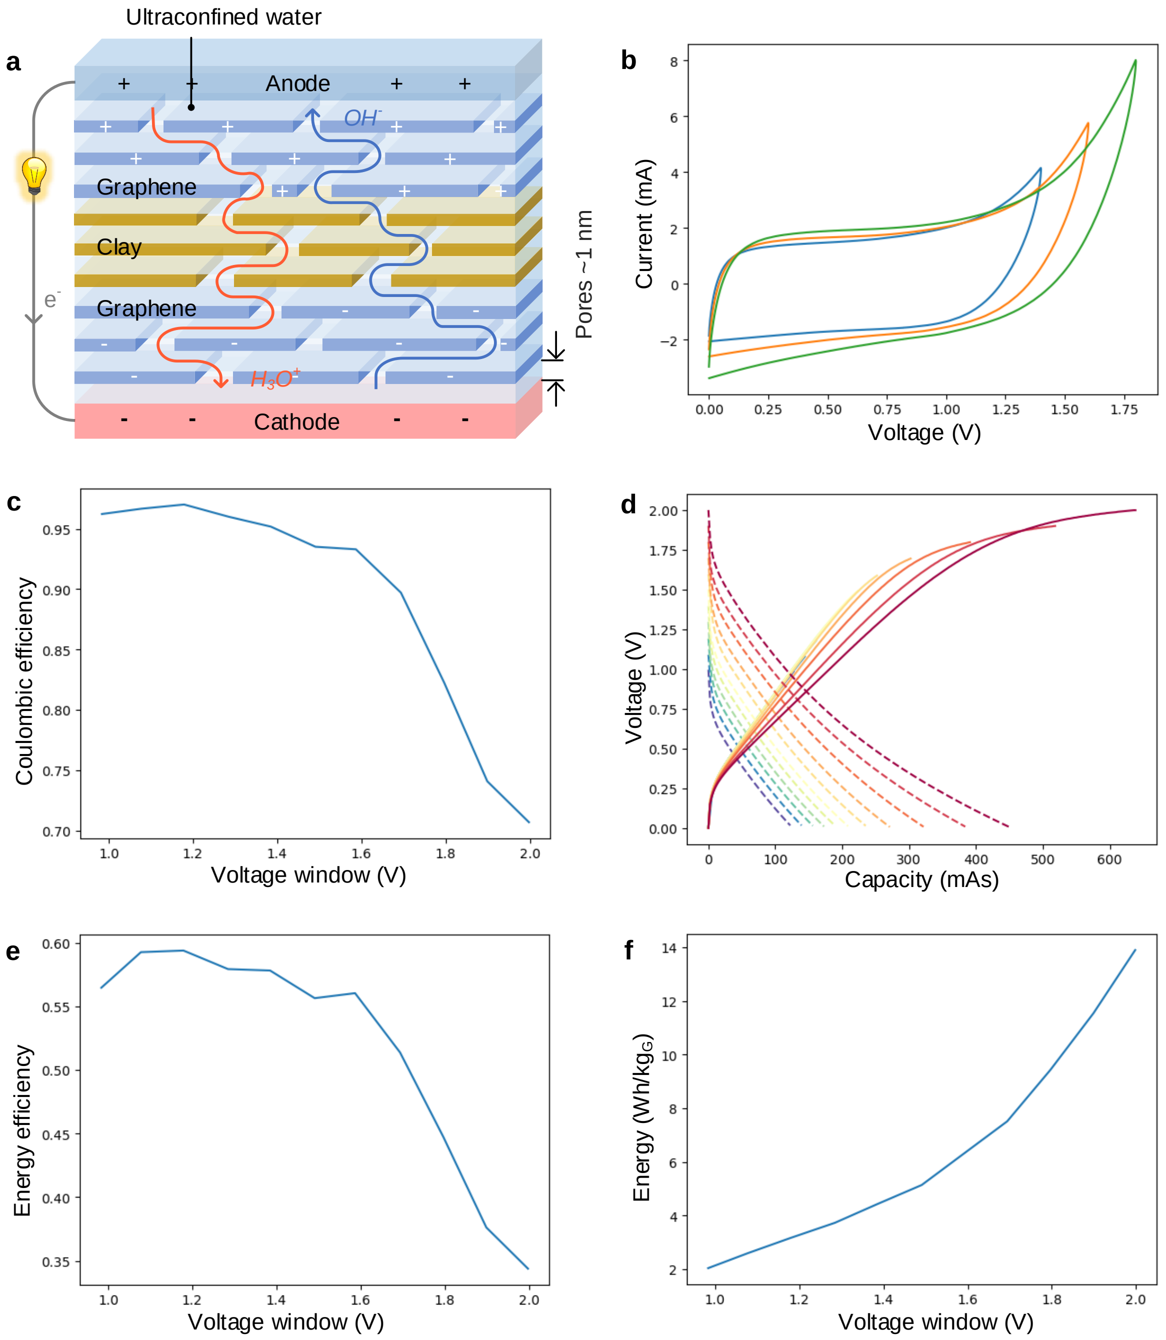


**Fig. S13. Test for the hydrogen evolution reaction** (HER). (a) Schematic representation of the blue battery cell. (b, d) Current-voltage characteristics and charge-discharge curves at different cut-off voltages. (c, e, f) Coulombic efficiency, energy efficiency, and specific energy of the cell as functions of the working voltage window. The trade-off voltage is around 1.65–1.70 V. The HER threshold is approximately 1.65 V, which is higher than the 1.23 V of bulk water.

## 2. Battery characterization

We characterized the cell using cyclic voltammetry (CV) and charge-discharge (CD) tests. In the CV measurements, the current was monitored while varying the voltage at a fixed rate. In contrast, during the CD tests, the voltage was adjusted while maintaining a constant current. CV measurements were employed to calculate the capacitance, *C*, using the following equation:

$$C = \frac{\int idv}{2\mu m \varDelta V}, \qquad \text{(S1)}$$

where *i* and *v* are the current and potential in the CV test, $\mu$ is the scan rate in V/s, m is the mass of active materials in grams, $\varDelta V$ is the voltage (potential) window during discharge in V, *I* is the constant discharge current in A, and $\varDelta t$ is the discharge time in seconds. An example of the results can be seen in Fig. S12.

CD curves were used to calculate the energy density, E, using the formula:

$$E = \int_{DC} \frac{IUdt}{m}, \qquad \text{(S2)}$$

and the power density, P, by:

$$P = \frac{E}{\varDelta t}. \qquad \text{(S3)}$$

An example of these results is provided in Fig. S15. The energy and coulombic efficiencies were determined from the CD and CV tests by dividing the output by the input energy and charge. These results are presented as percentages in Fig. S15. Finally, the long-term charge-discharge, and the self-discharge assessment test were performed. The results are given in Figs. S16 and S17.

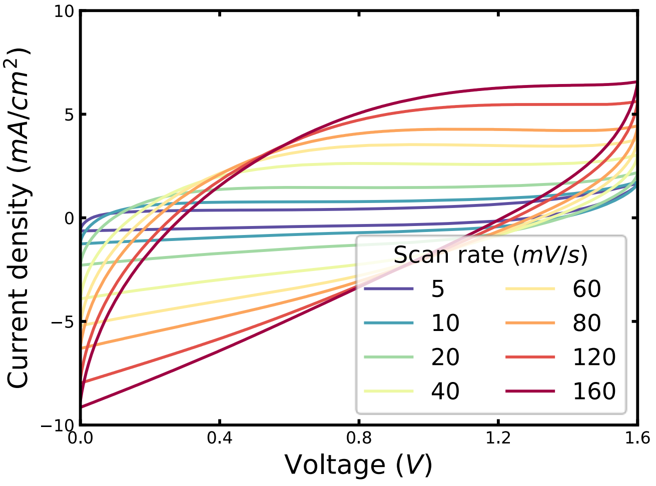


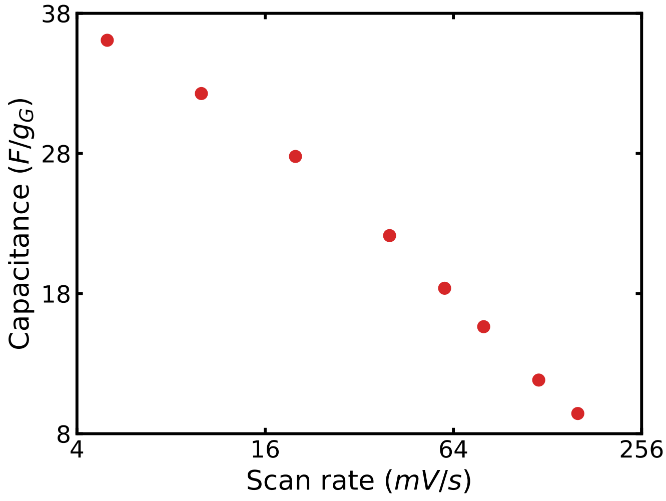


**Fig. S14.** Blue-battery cyclic voltammograms (top) and specific capacitance vs. scan rate, calculated according to Eq. (S1). The voltage window is ΔV = 1.6 V.

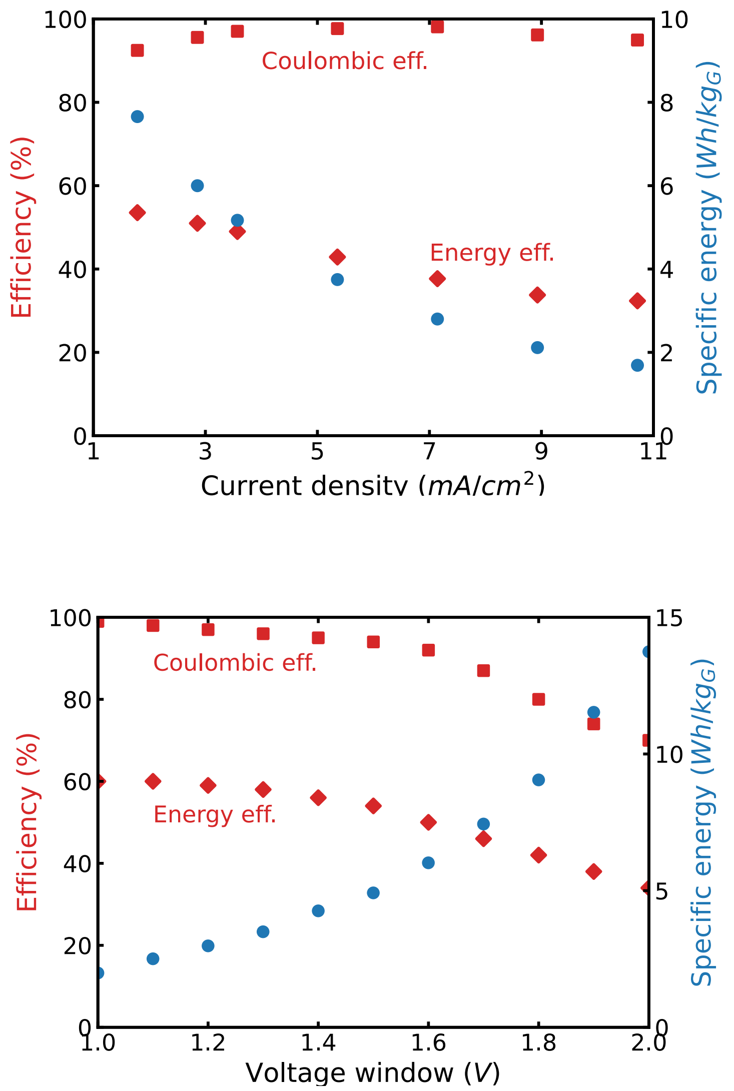


**Fig. S15.** Coulombic and energy efficiencies, as well as specific energy of the blue battery, at different current densities (top) and voltage windows (bottom).

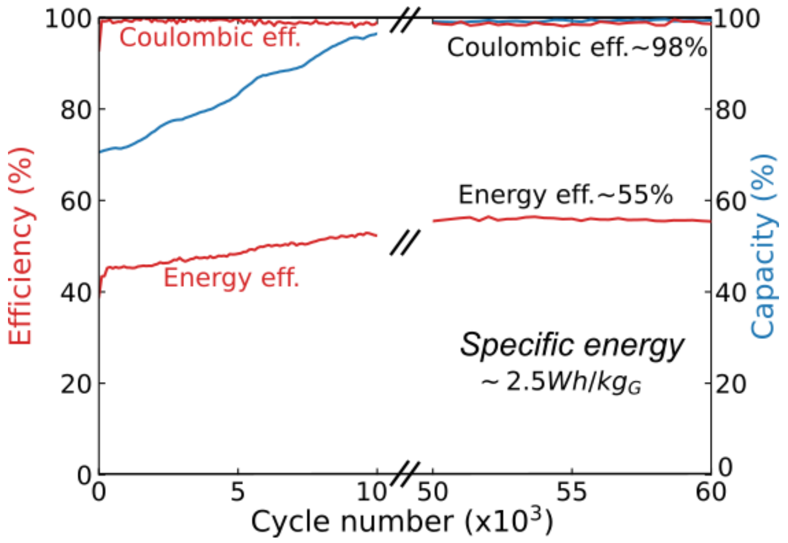


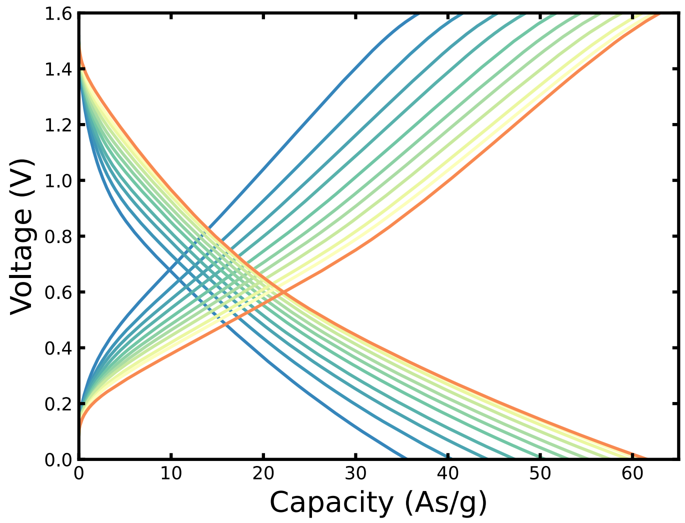


**Fig. S16. Long-term stability test.** The figure shows the evolution of the blue battery's efficiency, capacity, and specific energy over more than 60,000 cycles. The initial period exhibits an "annealing" effect, likely due to the electrowetting of nanopores. The bottom graph displays the progression of the charge-discharge curves, with blue representing the initial cycles and red representing the final cycles.

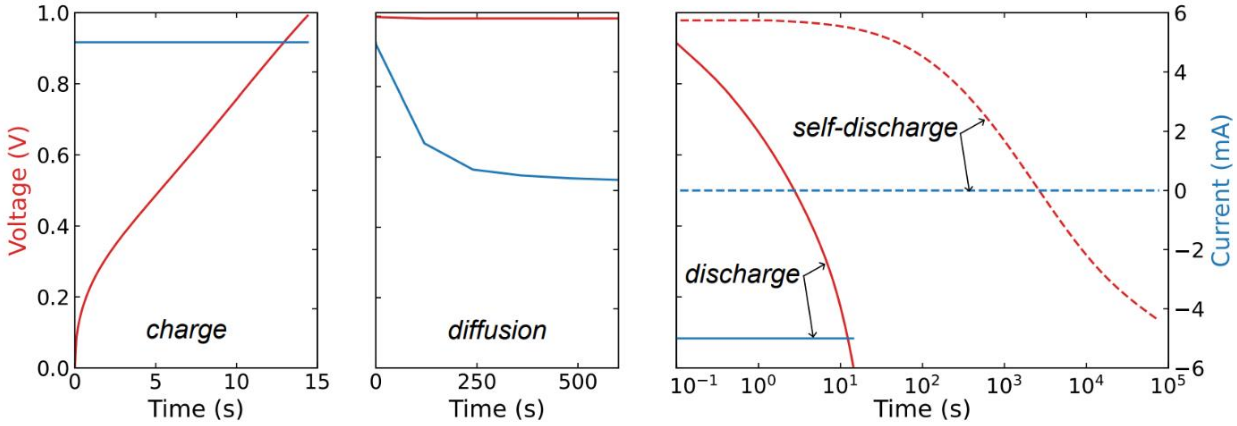


**Fig. S17. Self-discharge assessment.** The blue-battery charge phase with a fixed current (left), the diffusion phase with a variable current to maintain a constant voltage (middle), and the discharge phase (right), show both load discharge (solid line) and self-discharge with no load (dashed line). Note the logarithmic scale for the time in the right graph. The self-discharge occurs at a rate four orders of magnitude slower than the load discharge, indicating that the system is suitable for short- to mid-term electricity storage as a backup or an energy reserve, or a system where the fast charge-discharge and high power are needed, such as fast frequency control in the grid, or a regenerative brake system.

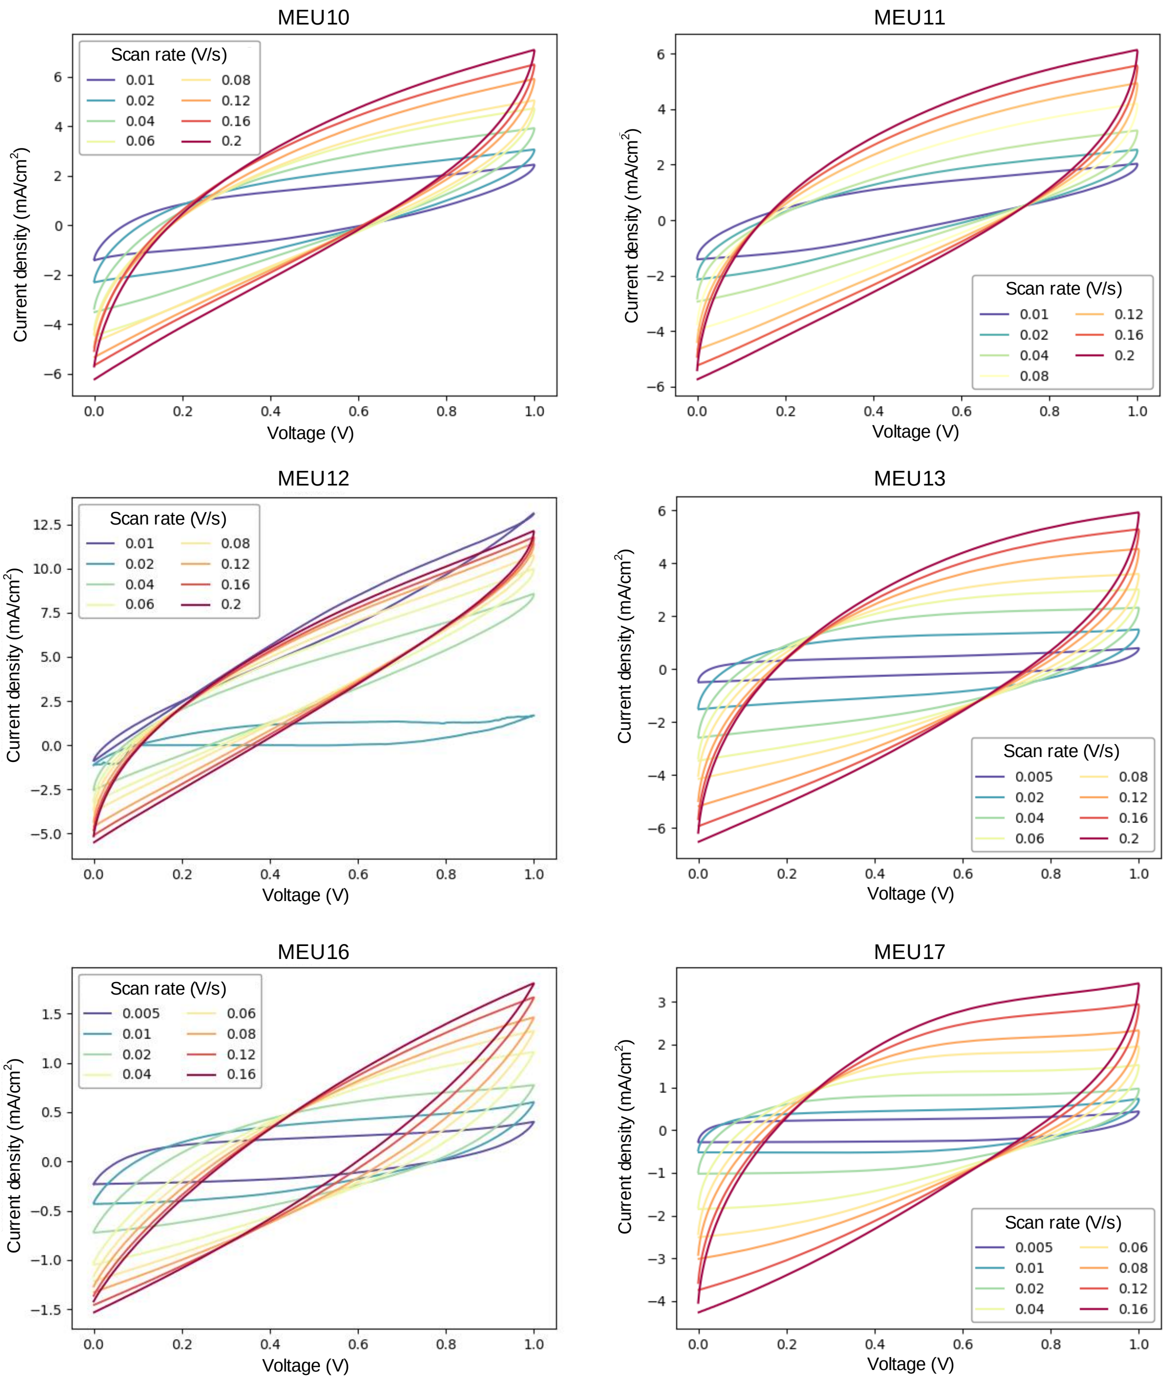


**Fig. S18.** Cyclic voltammograms for several different MEUs (see the number on top of the panels) at different scan rates. For MEU composition see Table 2.

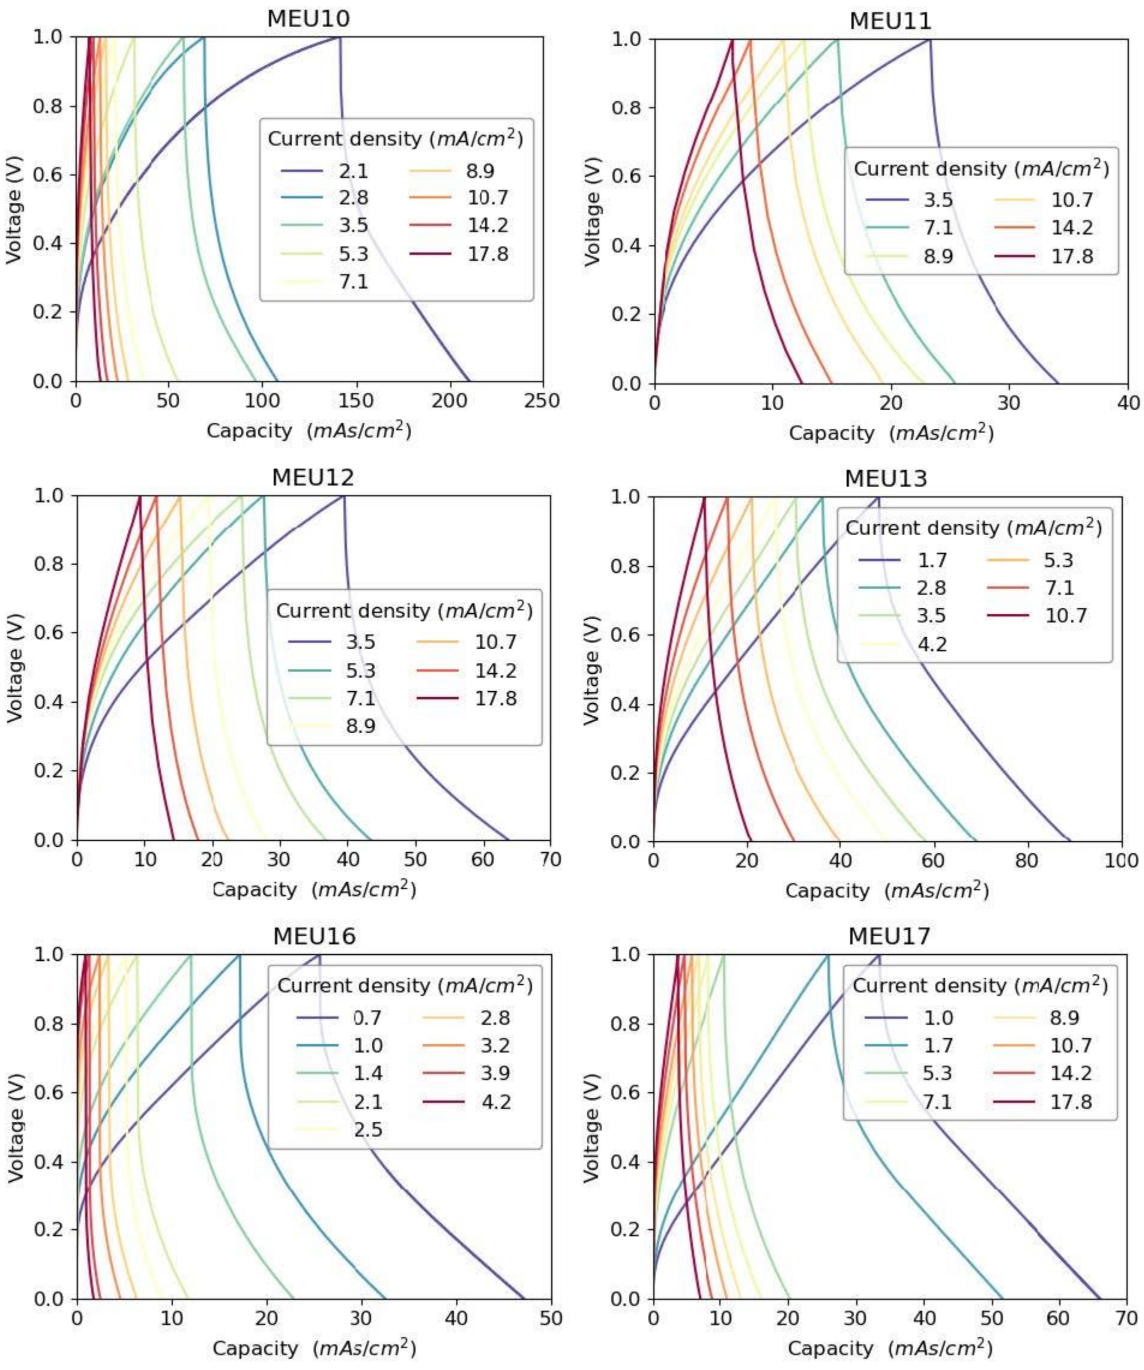


**Fig. S19.** Charge-discharge curves for several different MEUs (see the number on top of the panels) at different current densities. For MEU composition see Table 2.

**Table S2.** The list of membrane-electrode units (MEU) produced and tested in this study.

| MEU No | Electrodes | Separator | Sep. thickn. (μm) | Mass in the air (mg) | Wet mass (mg) | Mass gain (mg) |
|---|---|---|---|---|---|---|
| **1** | G 2mg/ml | BE 35 mg | 15 | 39.9 | 42.6 | 2.7 |
| **2** | G/BE 2ml/6mg | BE 35 mg | 15 | - | - | - |
| **3** | G/BE 1ml/10mg | BE 70 mg | 30 | 87.8 | 92.6 | 4.8 |
| **4** | G/BE 1ml/10mg | BE 35 mg | 15 | 58 | 61.9 | 3.9 |
| **5** | C/BE 5mg/5mg | BE 35 mg | 15 | - | - | - |
| **6** | G/BE/C 1ml/5mg/5mg | BE 70 mg | 30 | - | - | - |
| **7** | G/BE/C 1ml/10mg/5mg | BE 70 mg | 30 | 103.3 | 110.2 | 6.9 |
| **8** | G/BE/C 1ml/10mg/5mg | BE 35 mg | 15 | 51.7 | 54.5 | 2.8 |
| **9** | G/BE/C 1ml/10mg/5mg | BE 15 mg | 7 | 34.8 | 38.2 | 3.4 |
| **10** | G/BE 6ml/18mg | BE 35 mg | 20 | 125.6 | 253.7 | 128.1 |
| **11** | G/BE 10ml/18mg | BE 35 mg | 20 | 91 | 619.5 | 528.5 |
| **12** | G/BE 6ml/15mg | BE 15 mg | 10 | 77 | 521.8 | 444.8 |
| **13** | G/BE 6ml/15mg | BE 35 mg | 20 | 77 | 195.5 | 118.5 |
| **14** | C/G/BE 6ml/6ml/15mg | BE 35 mg | 20 | 89 | - | - |
| **15** | G/BE 6ml/15mg | BE 35 mg | 20 | 77 | - | - |
| **16** | G/BE 6ml/15mg | BE 35 mg | 20 | 120 | 236.2 | 116.2 |
| **17** | G/BE 6ml/15mg | BE 35 mg | 20 | 120 | 289.5 | 169.5 |
| **18** | G/BE 6ml/15mg | BE 35 mg | 20 | 120 | 208 | 88 |

Note: G=graphene, BE=Bentonite (Smectite).

## 3. Clay's electrical properties on compactness, clay type, and water content.

The conductivity of different clays was measured under wet and dry conditions (Fig. S20). Samples exposed to saturated water vapor and those saturated with water at high pressure were compared (Fig. S21). The effect of sample compactness under high pressure was explored (Fig. S22). It was found that the conductivity of clay is generally independent of sample compactness. Large water-filled pores were found to contribute less to conductivity compared to nanopores. Additionally, the electrical conductivity of clay reaches a maximum at a relatively low water content of approximately 30% and remains stable with higher water saturation. This suggests that ionic current primarily occurs within nanometer-sized interstitial slit pores rather than within larger micro-pores. These findings are consistent with previous studies, which report maximum proton conduction and water polarizability in pores around 1 nm [1, 2]. Thus, the interlayer channels in clay provide the necessary confinement to 'activate' the electrical properties of ultraconfined water.

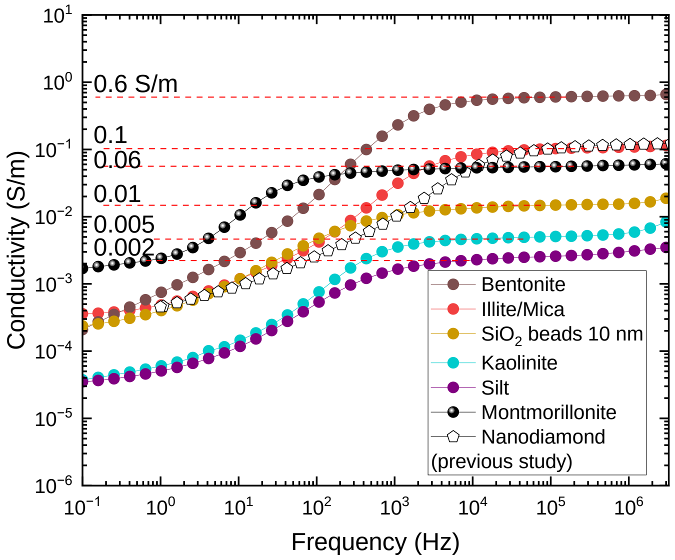


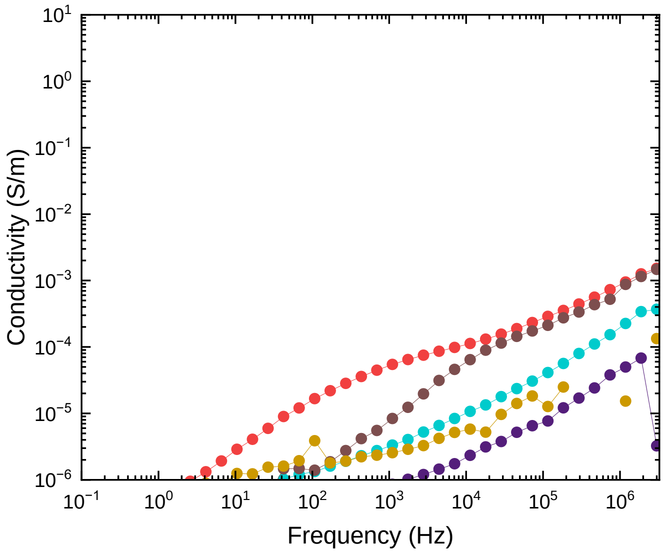


**Fig. S20. Proton conductivity of clays on water content.** Comparison of the proton conductivity data from Fig. 3d of the main text with that in other nanoporous materials, such as 10-nm silica beads ceramics, silt, and 5-nm nano-diamond ceramics (data from [1]). The top graph is for wet samples, the bottom graph is for the same dry samples. The dry samples were filled with water by long exposure to saturated water vapor, excluding contamination.

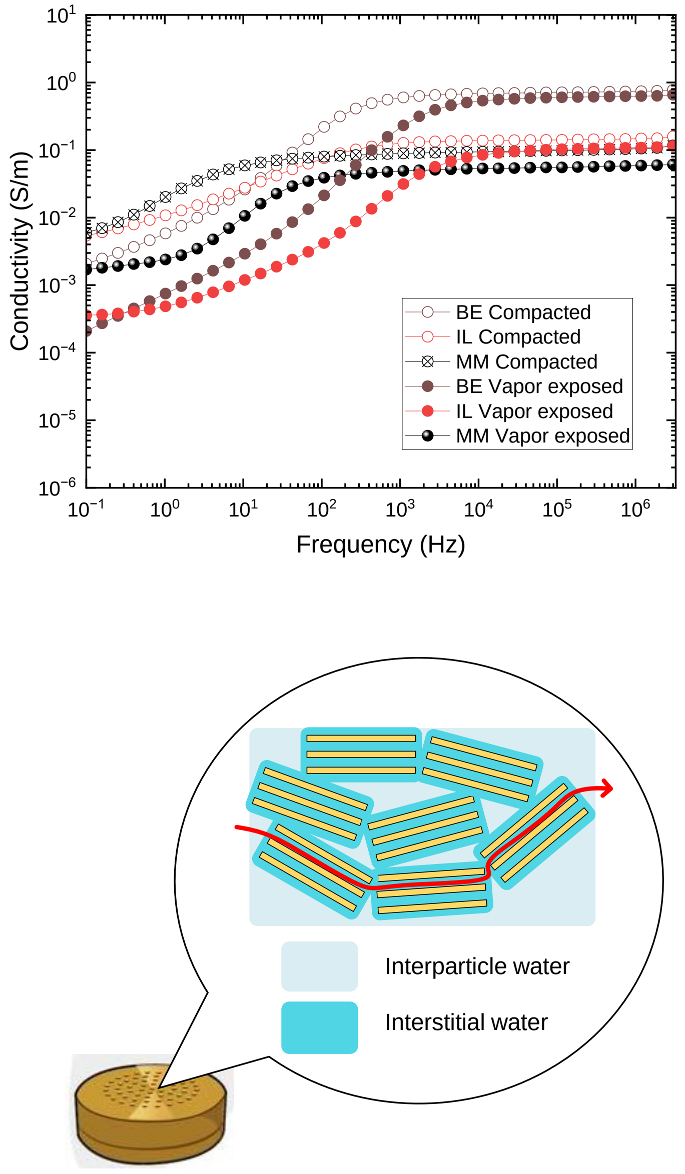


**Fig. S21. Proton conductivity of clays in micro and nanopores.** Comparison of electrical (proton) conductivity of the saturated-water-vapor-exposed clay samples (bentonite, illite, and montmorillonite) with that placed in liquid water under high pressure. The bottom picture shows the difference between the interstitial water between the clay crystal layers and the interparticle water in micropores between the clay particles. A minor difference between the two cases indicates that the conductivity originates from the nanopores rather than large micropores.

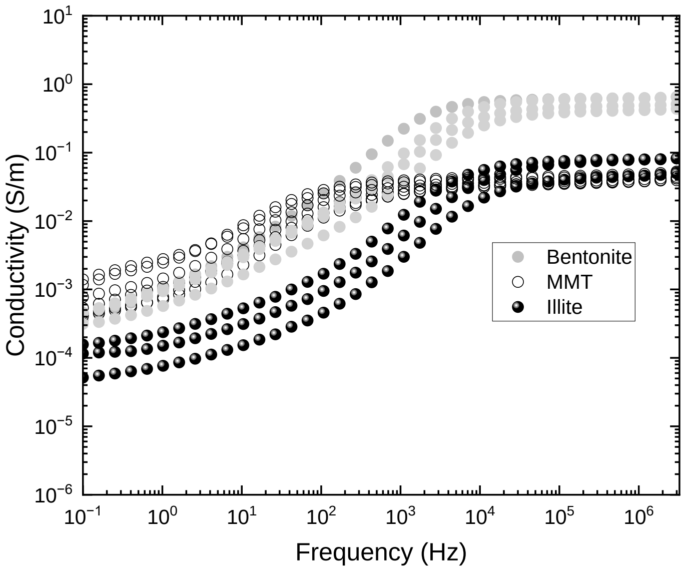


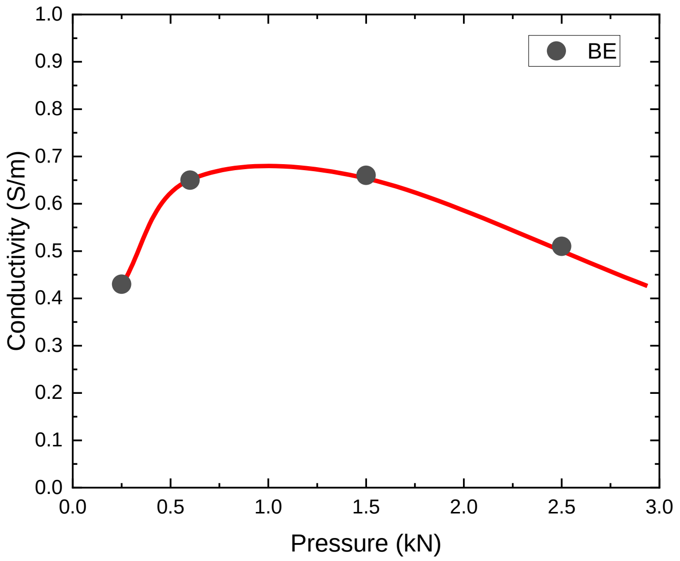


**Fig. S22. Proton conductivity of clays depending on the applied pressure.** The top graph shows the measurement of electrical conductivity at different pressures. The bottom graph shows the dependence of the DC conductivity plateau for bentonite clay. The red-curve fit shows that the pressure dependence of the clay proton conduction is weak. This confirms the results shown in Fig. S21 because pressure affects the large pores rather than nanopores.

## 4. SEM, TEM, and STEM imaging

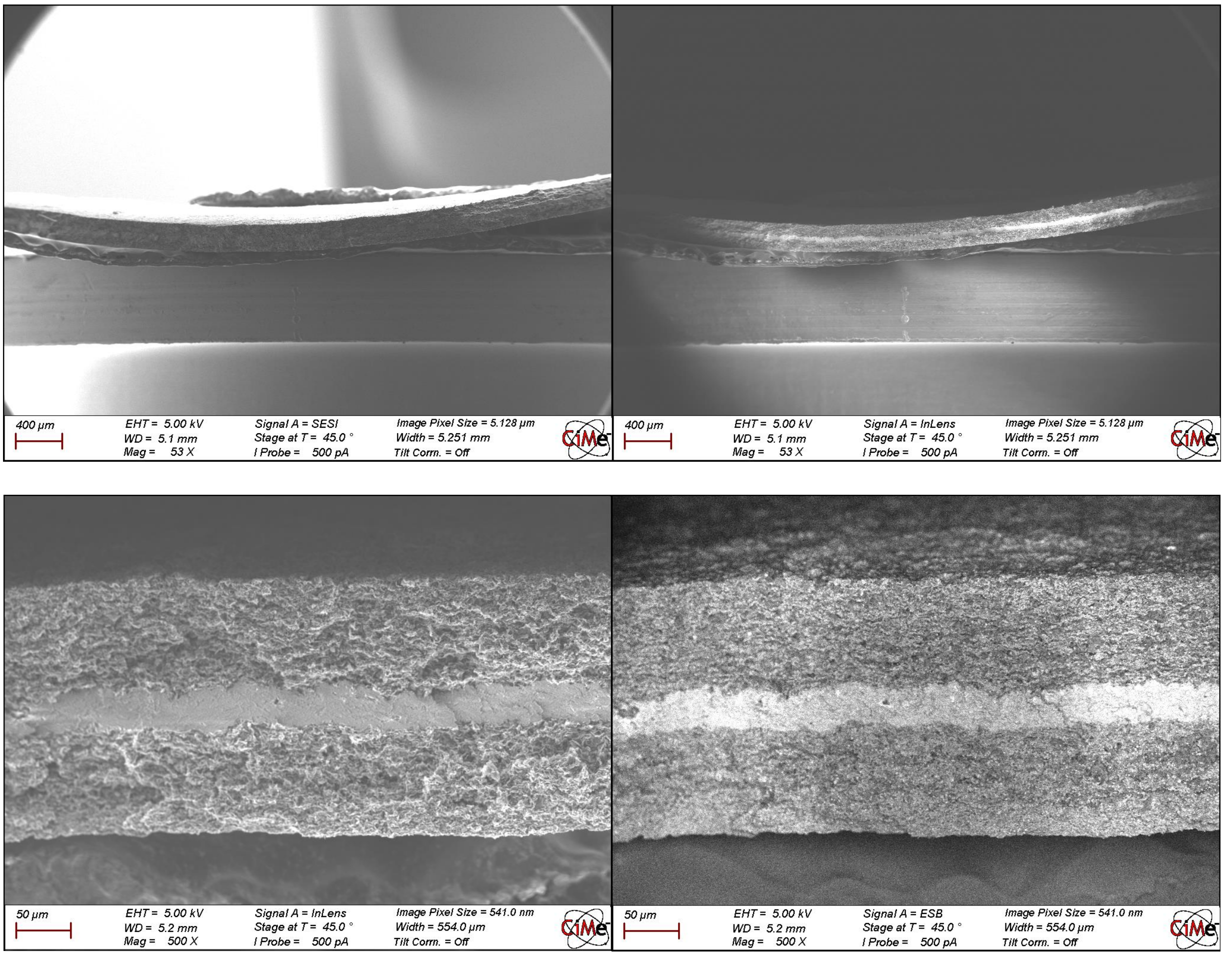


**Fig. S23.** SEM image of the cross-section of dry MEU10 (electrode thickness about 70 µm) at different resolutions (see scalebars and legends). Outer layers: 90% smectite, and 10% graphene. Inner layer: 100% smectite.

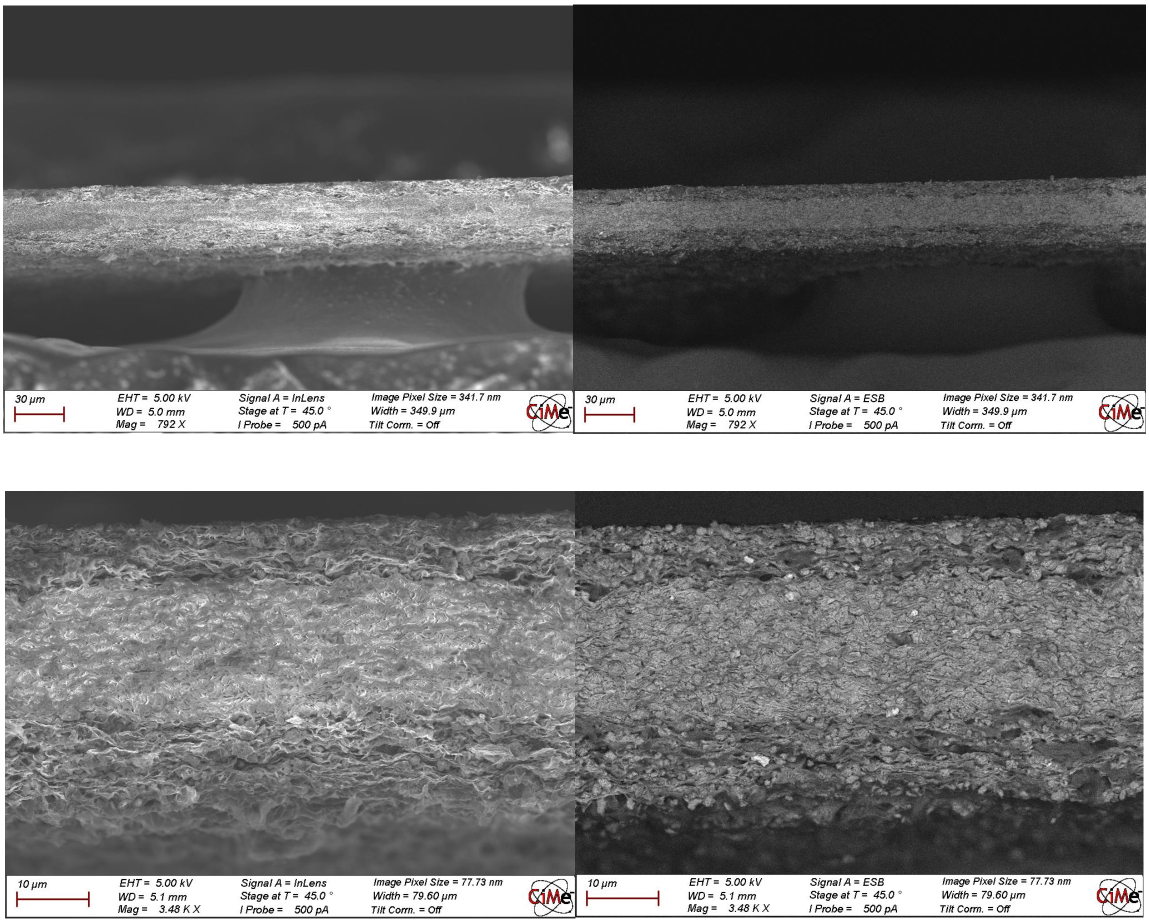


**Fig. S24.** SEM image of the cross-section of dry MEU4 (electrode thickness about 10 µm) at different magnifications (see scalebars and legends). Outer layers: 90% smectite, and 10% graphene. Inner layer: 100% smectite.

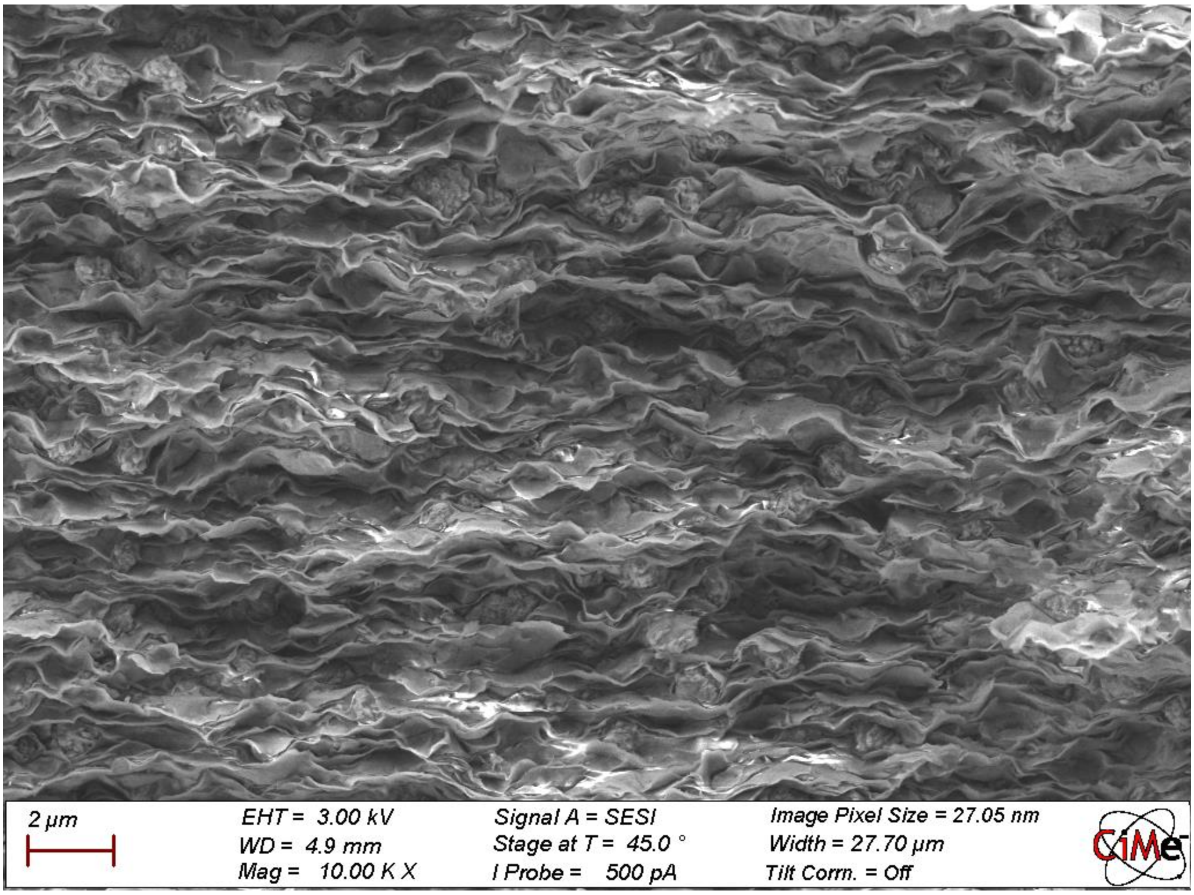


**Fig. S25.** SEM image of the cross-section of dry smectite membrane at different magnifications (see scalebars and legends).

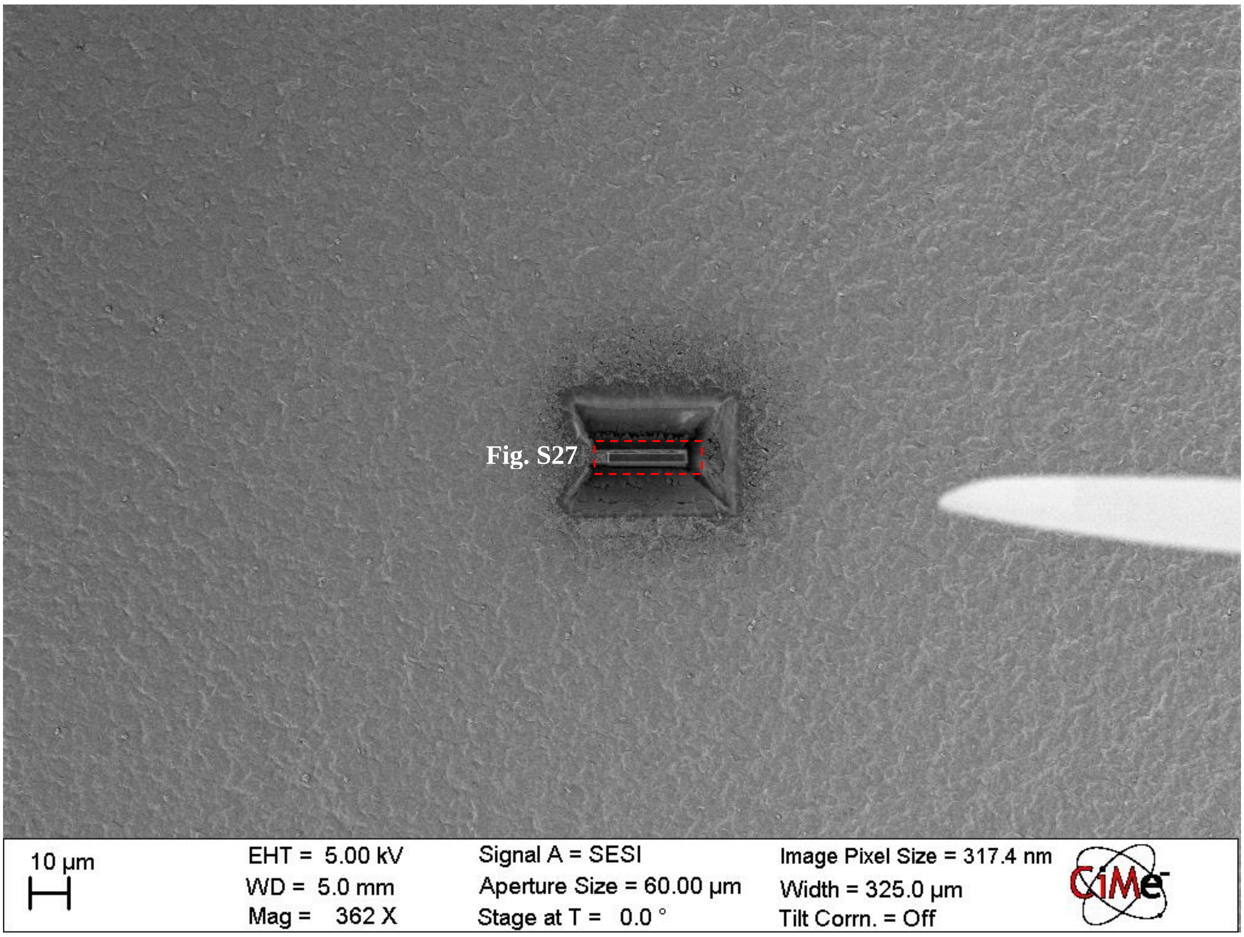


**Fig. S26.** SEM picture of the hole made by the Ga-focused ion beam (FIB) on the surface of a smectite membrane for TEM sample preparation. The middle part is lamella, the SEM and STEM images of which are shown in Figs. S27 and S28, respectively.

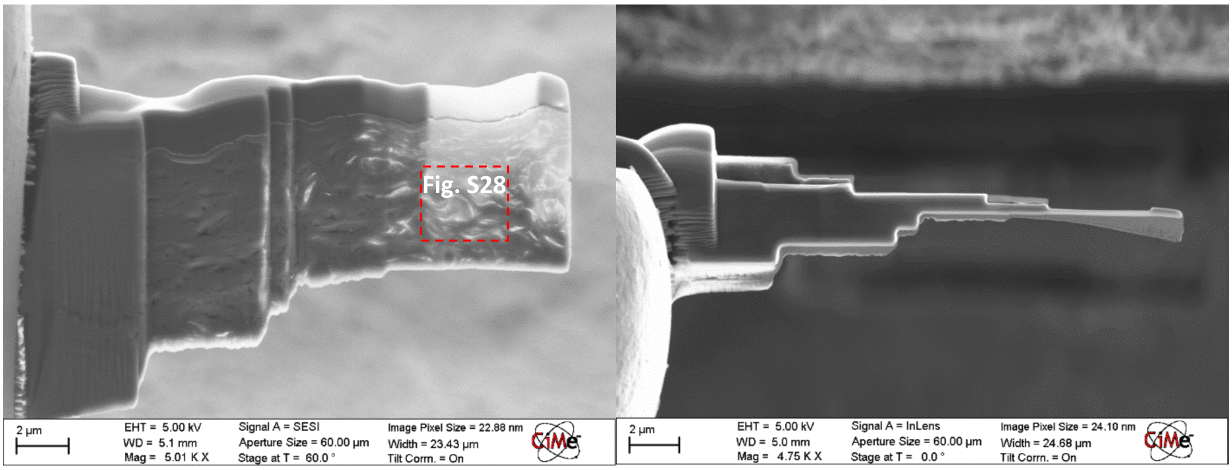


**Fig. S27.** SEM image of the lamella cut of smectite membrane from side (left) and top (right) views. The red square shows the part imaged by STEM in Fig. S28.

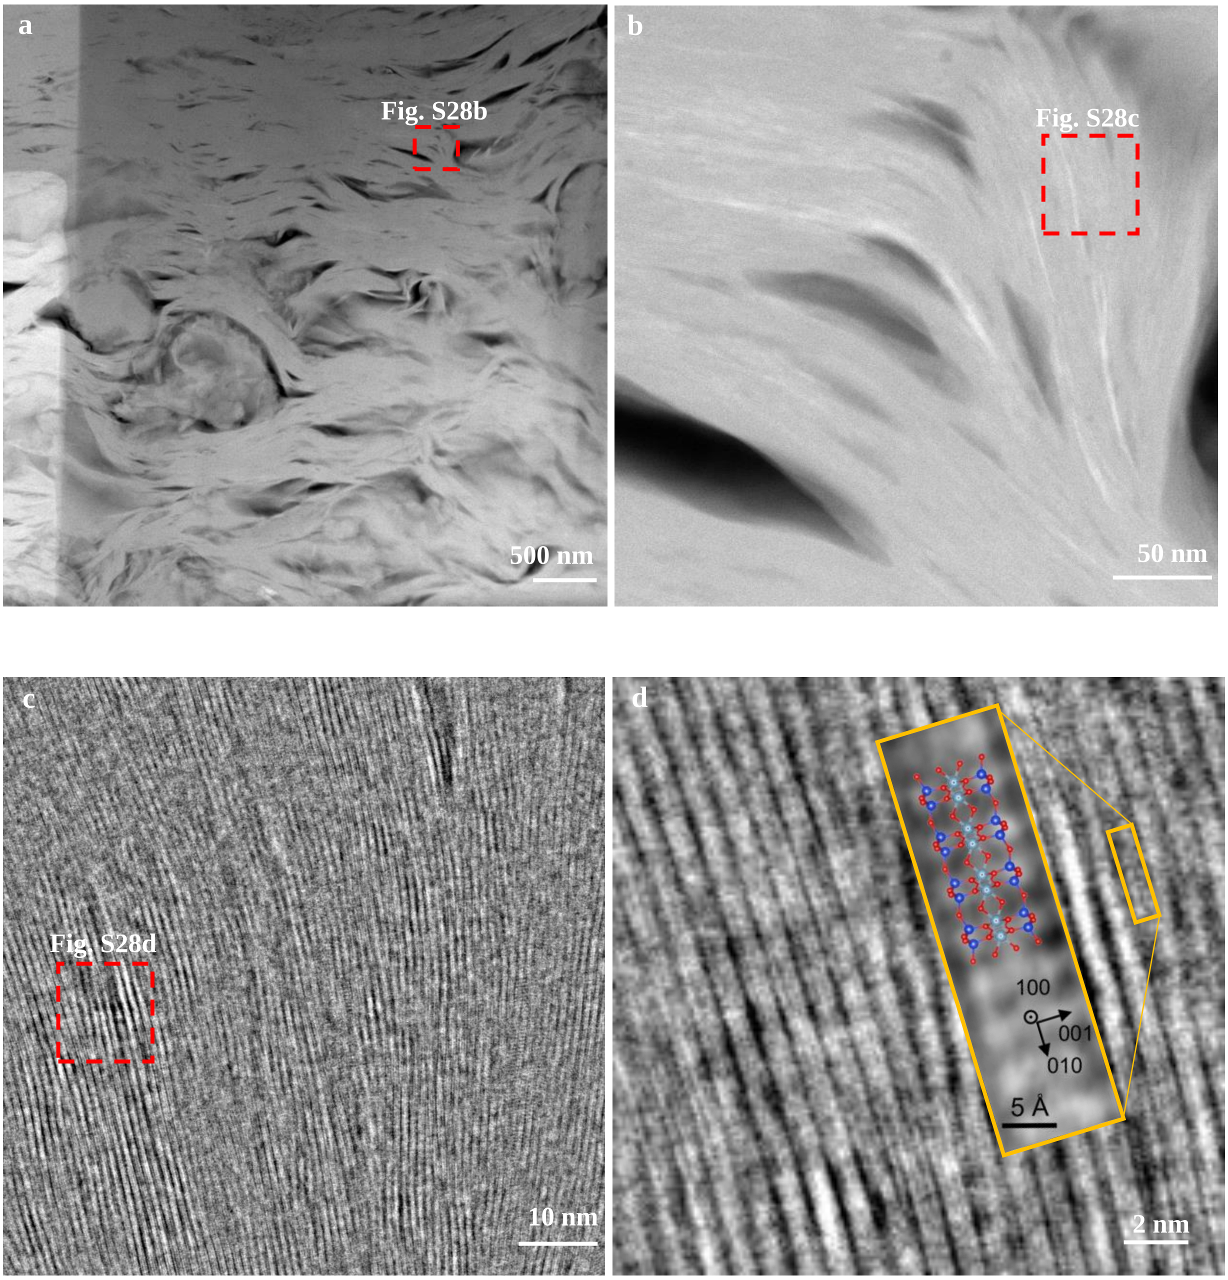


**Fig. S28.** STEM imaging of a cross-section of a smectite membrane at different resolutions (see scale bars). Red squares indicate the part enlarged on the next slide from left to right and top to bottom. (**a, b**) Annular dark-field (ADF) STEM images at lower magnification. (**c,d**) Integrated differential phase contrast (iDPC) STEM pictures, used to provide atomic-resolution images at the low-dose condition to prevent degradation of the crystal structure [3]. The inset shows the crystal structure overlapped on the atomic-resolution image. Red, blue, and cyan balls are for O, Si, and Al atoms, respectively.

**Table S3.** Comparison of the device of this study with other electricity retention technologies.

| | Li-ion Batteries | Lead-Acid Batteries | Pumped Hydro Storage | Flow Batteries | Standard Supercapacitors | **This study*** |
|---|---|---|---|---|---|---|
| Energy/Power density | High/Low | Moder./Low | Low/Moder. | Moder./Low | Moder./High | Moder./High |
| Lifecycle | 500-3000 cycles | 200-800 cycles | 30+ years | ~ 1000 cycles | > 5000 cycles | > 60000 cycles* |
| Charging time | hours | hours | days | hours | ms to minutes | µs to minutes* |
| Sustainability | Environmental impact, recycling challenges | Lead pollution, recycling challenges | Low environmental impact | Chemical pollution, habitat disruption | Moderate ecological impact, potential for recyclability | Natural materials, low environmental impact |
| Safety | Risk of thermal runaway, fire, and explosion | Risk of lead exposure, acid spills | Low risk, but potential for dam breach scenarios | Risk of chemical leakage | Low risk | Low risk |
| Dependence on raw materials | Rare earth elements (Li, Co, and Ni), subject to supply chain constraints and price fluctuations | Lead and sulfuric acid, subject to price fluctuations | Dependent on water resources, land availability, and regulatory approvals | Vanadium, zinc, iron, or other metal-based electrolytes, subject to supply chain constraints | Carbon-based materials, aluminum, and other metals, generally abundant and readily available | Uses readily and widely available materials, minimal risk of supply chain constraints |
| Applications | Portable electronics, Electric vehicles, Small-scale storage | Automobile starting and ignition batteries, Small-scale storage | Long-term energy storage from renewable sources | Backup power, short and long-term energy storage | Fluctuating loads (portable devices), Wind and photovoltaic systems peak loads shaving, Defibrillators, Transport braking energy recovery | Same as supercapacitors + Fast-frequency control, Biocompatible devices, Batteries for Mars colonization, Biodegradable batteries. |

**Based on lab-scale prototype tests.*

**References**


[1] Artemov, V.G., Uykur, E., Kapralov, P.O., Kiselev, A., Stevenson, K.J., Ouedane, H., Dressel, M.: Anomalously high proton conduction of interfacial water. J. Phys. Chem. Lett. 11, 3623–3628 (2020)

[2] Wang, R., Souilamas, M., Esfandiar, A., Fabregas, R., Benaglia, S., Nevison- Andrews, H., Yang, Q., Normansell, J., Ares, P., Ferrari, G., Principi, A., Geim, A.K., Fumagalli, L.: In-plane dielectric constant and conductivity of confined water. arXiv preprint 2407.21538 (2024)

[3] Bosch, E.G.T., Lazic, I., Lazar, S.: Integrated Differential Phase Contrast (iDPC) STEM: a new atomic resolution STEM technique to image all elements across the periodic table. Microsc. Microanal., 22, 306-307 (2016)

[4] Ito, A. and Wagai, R.: Global distribution of clay-size minerals on land surface for biogeochemical and climatological studies. Scientific Data, 4, 170103 (2017)
